# Supplementary material for: First observation and measurement of the branching fraction for the decay $B^0_s \to D_s^{*\mp} K^{\pm}$
Source: arXiv:1503.09086 source file (2015-07-01)
Supplement: Supplementary file 2 [file supplementary-app.tex]

\clearpage

\section*{Supplementary material for LHCb-PAPER-2014-064}

\begin{figure}[!htb]
  \begin{center}
    \includegraphics[width=\textwidth]{Fig1-S.pdf}
    \vspace*{-1.0cm}
  \end{center}
  \caption{\small
Comparison of the ratio of branching fractions
$\BF(\BsDsK)/\BF(\BsDsPi)$~presented in this paper to the previous \lhcb
result~\cite{LHCb-PAPER-2011-022} and results from \cdf~\cite{Aaltonen:2008ab}
and \belle~\cite{Louvot:2008sc}, along with the theoretical expectation as
determined in Ref.~\cite{DeBruyn:2012}. The red vertical line and band indicate
the theoretical lower bound, $\BF(\BsDsK)/\BF(\BsDsPi) \geq 0.080 \pm 0.007$,
while the blue vertical line and band represent the theoretical expectation
$\BF(\BsDsK)/\BF(\BsDsPi) = 0.086^{+0.009}_{-0.007}$.}
  \label{fig:RatioPlot}
\end{figure}

\begin{figure}[!htb]
  \begin{center}
    \includegraphics[width=0.7\textwidth]{Fig2-S.pdf}
    \vspace*{0.0cm}
  \end{center}
  \caption{\small
Comparison of branching fraction measurements for \BdDsK. The vertical dashed
line indicates the weighted average of the three measurements.}
  \label{fig:BRDsKPlot}
\end{figure}
\clearpage
